# Supplementary material for: RoboStep: Robot Rewards Benefit from Tracking Task Progress Step by Step
Source: arXiv:2611.39097 source file (2026-11-28)
Supplement: Supplementary file 2 [file related_work.tex]

\begin{table}[htbp]
\centering
\caption{\textbf{\textit{TODO}} Comparison of robot reward and simulation-privileged learning approaches. This is a simplified version and the completed version is provided in Appendix~\ref{app:full-related-work}}
\label{tab:related_work}
\fontsize{6.0}{6.6}\selectfont
\setlength{\tabcolsep}{0.85pt}
\renewcommand{\arraystretch}{0.95}
\begin{tabularx}{\linewidth}{@{}
L{0.55in} L{0.66in} L{0.70in} L{0.52in} c L{0.68in}
L{0.40in} L{0.52in} L{0.40in} c Y@{}}
\toprule
\makecell[l]{\textbf{Previous}\\\textbf{Work}} &
\makecell[l]{\textbf{Reward /}\\\textbf{Signal}} &
\makecell[l]{\textbf{Supervision /}\\\textbf{Source}} &
\makecell[l]{\textbf{Task}\\\textbf{Structure}} &
\makecell[c]{\textbf{Per-}\\\textbf{sist.}} &
\makecell[l]{\textbf{Transition /}\\\textbf{Verification}} &
\makecell[l]{\textbf{Target}\\\textbf{data}} &
\makecell[l]{\textbf{Policy}\\\textbf{use}} &
\makecell[l]{\textbf{Real}\\\textbf{use}} &
\makecell[c]{\textbf{R2S2R}} &
\textbf{Scope} \\
\midrule

\multicolumn{11}{@{}l}{\textit{Visual progress rewards for robot learning}}\\[-1.3pt]
LIV~\citep{liv2023} &
goal value / $\Delta V$ &
time order + goal/outcome &
flat global value & \xmark & \NA &
target-domain tuning &
planning / LCBC & rep. & \xmark &
sim+real \\

ReWiND~\citep{rewind2025} &
dense video progress &
target demos + time/rewind labels &
flat global progress & \xmark &
external success signal &
$\sim$5 demos/task &
IQL $\rightarrow$ SAC & online RL & \xmark &
8 sim + 5 real \\

SARM~\citepp{sarm2025} &
stage + local progress $\rightarrow$ global score &
target demos + human boundaries &
stages scalarized & \xmark &
stage re-inferred &
yes &
AW-BC / DiffQL & offline FT & \xmark &
real LH + sim \\

RoboReward~\citep{roboreward2026} &
episode 1--5 progress &
human scores + OXE truncation/time &
flat & \xmark &
terminal scoring &
none for RM &
DSRL-SAC & online RL & \xmark &
3 sim + 2 real \\

TOPReward~\citep{topreward2026} &
$P(\mathrm{True}\mid$prefix$)$ &
frozen VLM token probability &
flat global completion value & \xmark & \NA &
none for RM &
AWR (50 demos/task) & offline AWR & \xmark &
130 eval; 6 real \\

Large Reward Models~\citep{lrm2026} &
relative / absolute progress + completion &
multi-source video + temporal weak labels &
flat multi-head & \xmark &
completion head &
none for RM &
Pi0.5 + PPO & filtered BC & \xmark &
LH sim + real \\

RoboMeter~\citep{robometer2026} &
frame progress + success + preference &
RBM-1M: time labels + failure preferences &
manual stages + global progress & \cmark &
success head advances stage &
none for RM &
SAC, DSRL, IQL & online RL & \xmark &
sim+real; 21 emb. \\

SOLE-R1~\citep{soler12026} &
absolute progress $p_t$ &
sim GT progress + temporal/reversal; SFT+RLVR &
flat global progress & \xmark & \NA &
none &
SAC/DrQv2 from scratch & online RL & \xmark &
24 unseen; sim+real \\

ProcVLM~\citep{procvlm2026} &
stage-aware continuous progress &
VLM procedure labels on successful videos &
stages scalarized & \xmark &
stage inferred from video &
none for RM &
reward-weighted FT & offline FT & \xmark &
real LH \\

STDR~\citep{stdr2026} &
stage-transition + within-stage progress &
30 expert videos/task; auto stage labels &
stage-aware dense scalar & \xmark &
learned stage discriminator &
30 demos/task &
PPO from scratch & reward eval. & \xmark &
14 sim + real eval. \\

WVM~\citep{wvm2026} &
distributional value / progress chunk &
time weak + rewind / human-linear labels &
flat global value & \xmark & \NA &
none for RM &
AWR / filtered BC & offline FT & \xmark &
15 bench; 6 downstream \\

\midrule
\multicolumn{11}{@{}l}{\textit{Programmatic and structured reward design}}\\[-1.3pt]
Reward Machines~\citep{rewardmachines2018} &
event-conditioned executable reward &
manual automaton + event labels &
persistent RM & \cmark &
programmatic event predicate &
task spec. & RL & \NA & \xmark &
general RL \\

Text2Reward~\citep{text2reward2024} &
executable shaped code &
task text + env API/state &
mostly flat code & \xmark & \NA &
none & online RL & \NA & \xmark &
sim robot control \\

Eureka~\citep{eureka2024} &
executable shaped code &
task text + env source + fitness feedback &
mostly flat code & \xmark &
reward reflection, not runtime transition &
none; task search & PPO & \NA & \xmark &
29 envs; 10 morph. \\

Code-as-Reward~\citep{codeasreward2024} &
subtask completion programs + bonus &
VLM decomposition + trajectory verification &
ordered persistent subtasks & \cmark &
compiled completion predicate; offline verify &
2 expert + 100 random &
RL + auxiliary rewards & \NA & \xmark &
MiniGrid, PandaGym, CLIPort \\

PRM4RL~\citep{prm4rl2025} &
local subprogress $\rightarrow$ global potential &
task text + simulator state/API &
staged then scalarized & \xmark &
$\Psi(s)$ re-classifies from privileged state &
none & online RL & \NA & \xmark &
sim manipulation \\

ARM-FM~\citep{armfm2026} &
auto-generated reward machine &
language + env API + FM reasoning &
persistent RM & \cmark &
programmatic event-labeling function &
none & compositional RL & \NA & \xmark &
sim; zero-shot comp. \\


Phys2Real~\citep{phys2real2026} &
sim-privileged physical parameters &
VLM prior + RMA interaction history & \NA & \NA &
uncertainty-weighted fusion &
real image/history &
PPO in sim & deployment & \cmark &
2 sim + 2 real \\


\midrule
\textbf{RoboStep (ours)} &
\textbf{stage-local dense + boundary reward} &
\textbf{task/API for local code; VLM for semantic completion} &
\textbf{persistent compiled RM} & \cmark &
\textbf{online semantic gate + reversible rollback} &
\textbf{no human reward demos} &
\textbf{online visual RL / PPO} &
\textbf{sim$\rightarrow$real} & \cmark &
\textbf{rigid, artic., deform.} \\
\bottomrule
\end{tabularx}
\vspace{-1mm}
\end{table}
